# Supplementary material for: Falling Trees: A Model Class for Interpretable Risk Prioritization
Source: arXiv:2609.23780 source file (2026-09-20)
Supplement: Supplementary file 1 [file approximate_rset.tex]

\begin{itemize}
    \item Approximating the falling tree Rashomon set using SPLIT \cite{babbar}. Runtime before vs after. 
\end{itemize}
