# Supplementary material for: Falling Trees: A Model Class for Interpretable Risk Prioritization
Source: arXiv:2609.23780 source file (2026-09-20)
Supplement: Supplementary file 2 [file rset_of_frls.tex]

\begin{itemize}
    \item Describe FRAME as a baseline and how it relates to the algorithm in \cite{chaofan}. 
    \item Runtime theorem for FRAME from previous paper
\end{itemize}
