# Supplementary material for: Falling Trees: A Model Class for Interpretable Risk Prioritization
Source: arXiv:2609.23780 source file (2026-09-20)
Supplement: Supplementary file 3 [file rule-list-comparisons.tex]

% \todo[inline]{modify to make sense in context of falling trees rather than frls}
% We now discuss the method proposed by \citet{rulesets} and our attempts to run their method as a baseline for generating Rashomon sets of FRLs. \citet{rulesets} proposes an algorithm for finding the Rashomon set of the related hypothesis space of \textit{rule sets}. A rule set is similar to a rule list, but predicts positively if and only if any rule in the set is satisfied. FRLs can be viewed as rule sets that have order imposed to satisfy the falling constraint. Thus, FRLs are a constrained subset of rule lists, which are themselves subsets of decision trees, which are subsets of rule sets. We found that, with the same parameters, finding the Rashomon set of rule sets gave us an identical set of FRLs as \treefarms, but took much longer. We could not find a public code implementation of the \texttt{CORELSEnum} algorithm by \citet{mata2022computing}.
